# Supplementary material for: Model Selection, Adaptation, and Combination for Transfer Learning in Wind and Photovoltaic Power Forecasts
Source: arXiv:2204.13293 source file (2022-07-18)
Supplement: Supplementary file 5 [file nrmse_PVREAL_gbrt.tex]

\begin{tabular}{|l|r|r|}
\toprule
{} &   GBRT &  PVPhysical \\
\#Days &        &             \\
\midrule
% \midrule
7              &  \textbf{0.133} &       0.137 \\
14             &  \textbf{ 0.120} &       0.137 \\
30             &   \textbf{0.112} &       0.137 \\
60             &   \textbf{0.107} &       0.137 \\
90             &   \textbf{0.105} &       0.137 \\
365            &   \textbf{0.091} &       0.137 \\
\bottomrule
\end{tabular}
